# Supplementary material for: Generative Compression
Source: arXiv:1703.01467 ancillary file (2017-06-04)
Supplement: Supplementary file 1 [file CompressionSupp.pdf]

# Generative Compression – Supplementary Material

## 1 Additional Image Compression Results

As generative models approximate the data distribution, they have the potential to identify important features and properties of interest in the data. Due to this property, we believe images compressed using generative compression will deteriorate gradually in visual quality as compression factors increase. This is reflected in Figure 1, which shows select samples from the CelebA dataset [1] and Outdoor MIT Places dataset [2] at varying compression levels. It is clear that NCode compressed images exhibit graceful degradation and further the images look realistic and devoid of unnatural artifacts at even $\sim 1000$-fold compression. It is interesting to note that as compression levels rise, the source of errors is principally incorrect features, such as erroneous color or pose.

**CelebA** | **Outdoor MIT Places**

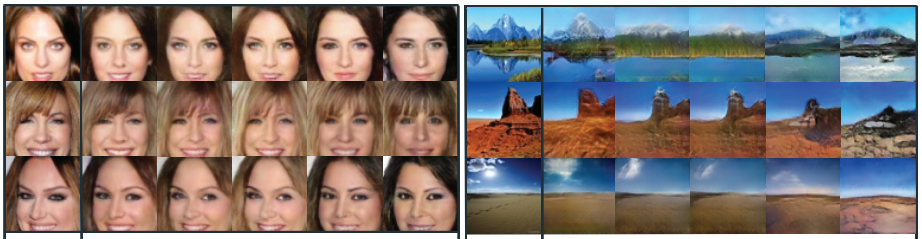

| | (a) CelebA | | | | | | (b) Outdoor MIT Places | | | | | |
|---|---|---|---|---|---|---|---|---|---|---|---|---|
| Bits/Pixel | 17 | 0.122 | 0.098 | 0.049 | 0.024 | 0.012 | 16 | 0.122 | 0.098 | 0.049 | 0.024 | 0.012 |
| PSNR | | 20.72 | 20.33 | 19.35 | 18.79 | 14.97 | | 19.32 | 18.96 | 18.24 | 17.34 | 12.13 |
| SSIM | | 0.740 | 0.723 | 0.700 | 0.679 | 0.543 | | 0.574 | 0.552 | 0.538 | 0.679 | 0.340 |

(a) (b)

Figure 1: A comparison of image reconstruction using NCode at different compression factors for (a) CelebA [1] and (b) Outdoor MIT Places [2] datasets in the low bits/pixel regime. In panels (a) and (b), the first column shows randomly sampled dataset images. The subsequent columns contain compressed images at different compression levels ranging from $0.012$ to $0.122$ bits/pixel.

As discussed in Section 5 of the paper, while our results serves as a proof-of-concept, it is currently tricky to extend these to larger images due to well-known GAN training instabilities. NCode uses a vanilla DCGAN, but even state-of-the-art GANs struggle when it comes to larger ($256 \times 256$ images or bigger). In Figure 2, we demonstrate the performance of NCode on larger and more challenging ImageNet images against traditional JPEG and JPEG2000 techniques. At high compression factors, JPEG/2000 lead to unnatural image artifacts even for larger images, albeit at slightly lower bits/pixel than thumbnail images. While the GAN based approach does not do as well for larger images when compared to smaller $64 \times 64$ images yet, these preliminary results are indicative of the potential of generative compression. Further, the improvement in NCode compressed images using a Wasserstein GAN instead of a basic DCGAN illustrates how the tremendous research effort towards bettering these models can boost generative compression.

## 2 Additional Video Compression Results

In addition to the MCode compression results for the KTH handwaving dataset shown in the paper, we benchmark on the KTH boxing dataset, shown in Figure 3(a). Comparing (b) MPEG to (c) frame-by-frame MCode, it is clear that our method provides higher quality results at a comparable compression level. Despite similar PSNR, the relative preservation of background texture and limb sharpness is noteworthy. Motivated by MPEG bidirectional prediction, MCode can produce greater

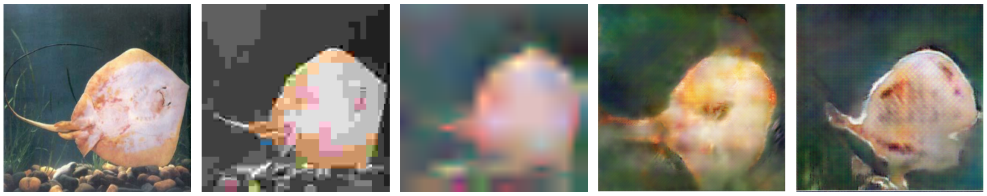


Figure 2: Comparison of larger image compression (256x256) from the difficult ImageNet dataset using traditional JPEG and JPEG2000 techniques, and proposed NCode algorithm. File header size was excluded from JPEG/2000 results for fairer comparison.

compression by interpolating between frames in latent space. This process is shown in Figure 3 (d-f). Frames transmitted and reconstructed using standard NCode are are omitted, with the remaining $N-1$ interpolated frames shown for (d) $N=2$, (e) $N=4$ and (f) $N=8$. These temporal correlations can be further leveraged by transmitting the Huffman-encoded difference between $\mathbf{z}^{(t)}$ and $\mathbf{z}^{(t+N)}$, leading to a further $20\%$-$50\%$ lossless compression on average. As shown in Figure 3, this can lead to order-of-magnitude reduction in bitrate over MPEG4 while providing more visually plausible sequences.

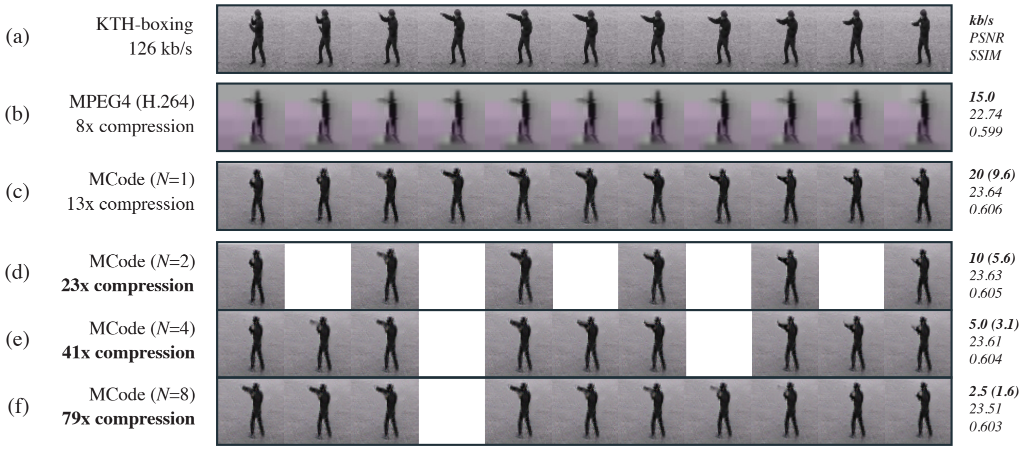


Figure 3: (a) Boxing video sequence randomly sampled from the KTH actions dataset [3]. Row (b) demonstrates the corresponding frame-by-frame reconstructions, bitrates and mean PSNR/SSIM metrics (averaged over the full test set) for MPEG4 (H.264). Row (c) shows the corresponding performance for MCode using $N=1$, i.e. applying image NCode frame-by-frame. Rows (d-f) demonstrate the extra performance than can be leveraged by linear interpolation between latent vectors $\mathbf{z}^{(t)}$ and $\mathbf{z}^{(t+N)}$ for (d) $N=2$, (e) $N=4$ and (f) $N=8$ (transmitted frames omitted). Bit rates are presented both before and after Huffman coding (parentheses).

## References

[1] Ziwei Liu, Ping Luo, Xiaogang Wang, and Xiaoou Tang. Deep learning face attributes in the wild. In *Proceedings of International Conference on Computer Vision (ICCV)*, 2015.

[2] Bolei Zhou, Agata Lapedriza, Jianxiong Xiao, Antonio Torralba, and Aude Oliva. Learning deep features for scene recognition using places database. In *Advances in neural information processing systems*, pages 487–495, 2014.

[3] Christian Schuldt, Ivan Laptev, and Barbara Caputo. Recognizing human actions: A local svm approach. In *Pattern Recognition, 2004. ICPR 2004. Proceedings of the 17th International Conference on*, volume 3, pages 32–36. IEEE, 2004.
